# Supplementary material for: On the analysis of scheduling algorithms for structured parallel computations
Source: arXiv:1810.10632 source file (2018-10-24)
Supplement: Supplementary file 1 [file appendix-3.tex]

\section{The Compare-And-Swap instruction}
\label{sec:cas-semantics}

\begin{algorithm}
  \caption{The CAS instruction}
  \label{algo:cas}
  \begin{scriptsize}
  \begin{algorithmic}[1]
   \Function{CAS}{$m, old, new$}
         \If{Memory[$m$]$\ = old$}
        \State Memory[$m$]$\ \gets new$\;
        \State \Return SUCCESS\;
      \Else\
         \State \Return FAILURE\;
      \EndIf
      \EndFunction
  \end{algorithmic}
  \end{scriptsize}
\end{algorithm}
